# Supplementary material for: Counterfactual Evaluation of Treatment Assignment Functions with Networked Observational Data
Source: arXiv:1912.10536 source file (2019-12-22)
Supplement: Supplementary file 1 [file appendix.tex]

\pagebreak
\section{Appendix*}

%\subsection{Essential Loss and Tractable Loss}
%We can rewrite the essential loss and the tractable loss as expectations  on different populations of the following 1-0 loss:
%\begin{equation}
%\label{eq:1-0}
%\mathcal{L}_{1-0}((\bm{x},\bm{t}),\left\{(\bm{x}',\bm{t}')\right\};f) = 1-\prod_{(\bm{x}',\bm{t}')}\mathds{1}(f(\bm{x},\bm{t})>f(\bm{x}',\bm{t}'))
%\end{equation}
%For each indivudual $i$, the essential loss can be formed as:
%\begin{equation}
%	|\mathcal{T}|\mathds{E}_{\bm{t}\sim Pr(\bm{t})}[\mathcal{L}_{1-0}((\bm{x}_i,\bm{t}),\left\{(\bm{x}_i,\bm{t}')\right\}_{\bm{t}'\not =\bm{t}};f)]
%\end{equation}
%While the tractable loss is:
%\begin{equation}
%	\mathcal{L}_{1-0}((\bm{x}_i,\bm{t}_i),\left\{(\bm{x}_j,\bm{t}_j)\right\}_{j\not =i};f)
%\end{equation}

\subsection{Machine}
All the experiments of this work are conducted on a desktop with 4 processors (AMD Ryzen 3.3GHz) with 64GB of RAM. The proposed model is programmed with
Python 3.6 mainly using Tensorflow\footnote{https://www.tensorflow.org/}, scikit-learn\footnote{https://scikit-learn.org/} and Numpy\footnote{http://www.numpy.org/}.

\subsection{Using POEM as a Baseline}
We modify the label used by the authors in their code because we aim to predict the optimal treatment. In particular, we replace the Hamming distance $\delta(\hat{\bm{t}}_i,\bm{t}_i)$ with negative outcome $-y_i$.
Then POEM would learn to minimize $-\hat{y}_i$ by predicting the optimal treatment.

\subsection{ACIC Benchmark}
Here, given the feature matrix $\bm{X}$ from the ACIC 2017 Challenge dataset, we formally describe how the treatments and outcomes are simulated:
\begin{equation}
\begin{split}
\bm{\kappa}_1 & \sim \mathcal{N}(\mu_{\kappa1},1);\; \bm{\kappa}_2 \sim \mathcal{N}(\mu_{\kappa2},1); \; \bm{\xi} \sim \mathcal{N}(\mu_{\xi},1); \;\eta=\mu_{\eta}, \\
f(\bm{x}_i) & = x_{i,1}+x_{i,43}+0.3(x_{i,10}-1),\\
\pi_j(\bm{x}_i) & = Pr(t_{i,j}=1) = \frac{\exp(\kappa_{1,j}f(\bm{x}_i)+\kappa_{2,j})}{\sum_{j'}\exp(\kappa_{1,j'}f(\bm{x}_i)+\kappa_{2,j'})},\\
\bm{t}_i & \sim Pr(\bm{t}_i=\bm{e}_j) =  [\pi_1(\bm{x}_i),...,\pi_{|\mathcal{T}|}(\bm{x}_i)] \\ % =  \underset{\bm{t}'\in\left\{\bm{e}_1,...,\bm{e}_{|\mathcal{T}|}\right\}}{\arg\max}<\bm{t}',\bm{\pi}(\bm{x}_i)>,\\
\mu(\bm{x}_i) & = -sin(g(\max\bm{\pi}(\bm{x}_i)))+x_{i,43},\\
\tau_j(\bm{x}_i) & = \xi_j(x_{i,3}x_{i,24}+(x_{i,14}-1)-(x_{i,15})-1),\\
\sigma_{y_i} &= \eta\sqrt{Var(\mu(\bm{x}_i)+<\bm{\pi}(\bm{x}_i),\bm{\tau}(\bm{x}_i)>)}\\
y_i & = \mu(\bm{x}_i) + \sum_j\tau_j(\bm{x}_i)t_{i,j}+\sigma_{y_i}\epsilon_i,\\
\end{split}
\end{equation}
where $a_{i,j}$ denotes the $j$-th dimension of the vector $\bm{a}_i$, <$\bm{a},\bm{b}$> signifies the dot product of the vectors $\bm{a}$ and $\bm{b}$, $\bm{e}_j$ is the one-hot vector with the $j$-th element as $1$, and $\max(\bm{a})$ refers to the maximal element in vector $\bm{a}$.
Following~\cite{hahn2018atlantic}, we set the parameters as $(\mu_{\kappa1},\mu_{\kappa2}) \in\left\{(0.5,0), (3,-1)\right\}$, $\mu_{\xi}\in\left\{1/3,2\right\}$, and $\mu_{\eta}\in\left\{0.25,1.25\right\}$.

\subsection{Twins Dataset}
Here, we explain how we sample a baby from each twins as the observed instance. In particular, we sample weights $\bm{u}\sim Uniform(-0.01,0.01)^{d}$ and noise $v_i\sim Gaussian(0,0.01)$. At the end, we sample $p_i\sim Bernoulli(\phi(\bm{u}^T\bm{x}_i+v_i))$ for each individual $i$. If $p_i=1$, we then choose the baby with heavier weight as the observed instance; otherwise, the lighter baby would be the observed instance.
%\subsection{Normal Learning to Rank (LETOR) Models}
%Here, we explain why normal LETOR models are not used as baselines.
%For pointwise LETOR models, we.
%For pairwise LETOR models, the difference between two concatenated instances of the same individual is always $concat([0]^d,\bm{t}-\bm{t}')$, so the model make personalized treatment decision. 
